# Supplementary material for: Understanding and engineering phonon-mediated tunneling into graphene on metal surfaces
Source: arXiv:1810.12082 source file (2018-10-29)
Supplement: Supplementary file 1 [file ligra_nl_si_revised.pdf]

# Supporting information: Understanding and engineering phonon-mediated tunneling into graphene on metal surface

J. Halle,*,† N. Néel,† M. Fonin,‡ M. Brandbyge,¶ and J. Kröger†

†Institut für Physik, Technische Universität Ilmenau, D-98693 Ilmenau, Germany

‡Fachbereich Physik, Universität Konstanz, D-78457 Konstanz, Germany

¶Center for Nanostructured Graphene, Department of Micro- and Nanotechnology, Technical University of Denmark, DK-2800 Kongens Lyngby, Denmark

E-mail: johannes.halle@tu-ilmenau.de

## 1 Experiment

### Experimental Methods

The experiments were performed with an STM operated at 6 K and in ultrahigh vacuum ($10^{-9}$ Pa). Tips were fabricated from chemically etched W wire coated *in situ* with a Au film. Ir(111) surfaces were prepared by $Ar^+$ bombardment and annealing in $O_2$ ($10^{-7}$ Pa). Graphene was epitaxially grown by thermal decomposition of $C_2H_4$.[1] The graphene-covered Ir(111) surface was exposed to Cs or Li sublimated from heated dispensers or to Ni from a hot filament at room temperature. Subsequent annealing ensured the efficient intercalation and the removal of adsorbed atoms on graphene. Only for the data presented in Figure 1e of the main manuscript Li was evaporated onto the hot sample at a temperature of 630 K. The Li coverage was progressively increased by deposition of additional Li. All STM images

were recorded in the constant-current mode with the bias voltage applied to the sample. Constant-height spectra of the differential conductance ($\mathrm{d}I/\mathrm{d}V$) were recorded by sinusoidally modulating the bias voltage ($6\,\mathrm{mV_{pp}}$, $6.3\,\mathrm{kHz}$) and measuring the current response of the junction with a lock-in amplifier. Intercalant coverages were determined by measuring the fraction of covered surface area in STM images and multiplying it with the fraction of carbon rings occupied with intercalant atoms. Based on the known atomic arrangement of the intercalated species, this fraction is 33 % for $(\sqrt{3} \times \sqrt{3})\,\mathrm{R}30^\circ$ Li[2] and 50 % for $(2 \times 2)$ Cs.[3] The highest coverage of the Li-intercalated sample was estimated from the evaporation time based on a calibration using the lower coverage data.

## Additional Spectroscopic Data for Li

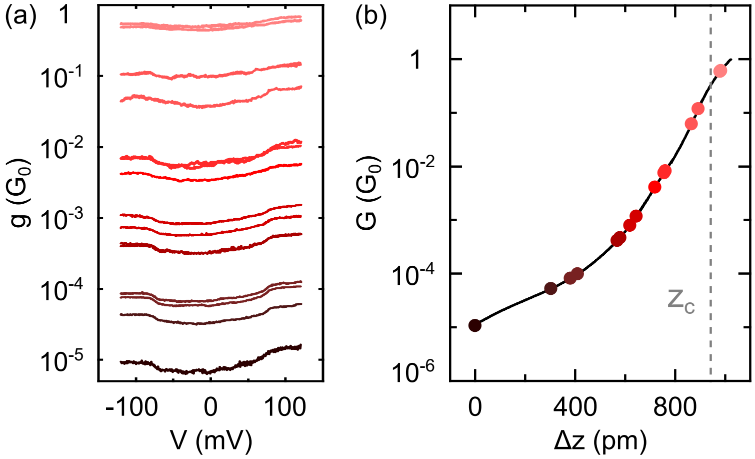


Figure S1: (a) Experimental $\mathrm{d}I/\mathrm{d}V$ ($g$) spectra of Li-intercalated graphene for increasing (bottom to top) junction conductance showing the progressive quenching of the graphene phonon gap. Closely spaced spectra reflect data acquired at tip approach and retraction. (b) Junction conductance $G$ as a function of the tip displacement $\Delta z$ with $z_\mathrm{c}$ the contact point (dashed line). $\Delta z = 0\,\mathrm{pm}$ is defined by $120\,\mathrm{mV}$, $100\,\mathrm{pA}$. Each dot marks the junction conductance at which spectra in (a) were acquired.

In analogy to Figure 3a of the main manuscript, Figure S1a shows $\mathrm{d}I/\mathrm{d}V$ data obtained for Li-intercalated graphene with increasing junction conductance (from bottom to top). Similar to the findings for Cs-intercalated graphene (Figure 3a) the phonon-induced gap is progressively quenched with increasing conductance and essentially vanishes at contact. A

typical conductance-versus-displacement curve is presented in Figure S1b. Compared to the Cs-intercalated sample (Figure 3b) the transition range ($400\,\mathrm{pm} \lesssim \Delta z < z_\mathrm{c}$) is extended, which hints at junction relaxations that start at lower conductance for the Li-intercalated sample, mediated by larger van der Waals interactions presumably due to a less sharp tip than in the Cs case.

The IETS signals of graphene phonons are absent on flat graphene on Ir(111). They exclusively appear above the nanostructures caused by Li intercalation. In these intercalated regions, $\mathrm{d}I/\mathrm{d}V$ spectra are virtually identical (Figure S2). Only at the very edges of the nanostructures the phonon signals vanish quite abruptly.

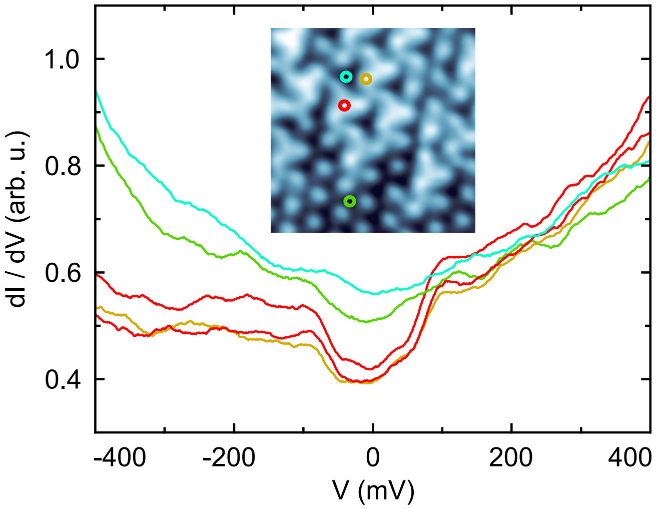


Figure S2: Spatially resolved $\mathrm{d}I/\mathrm{d}V$ spectra for a Li coverage of 0.15 ML. Inset: STM image (180 mV, 100 pA, $20 \times 20\,\mathrm{nm}^2$) of Li-intercalated graphene with indicated spectroscopy positions. The phonon-induced gap is best seen above intercalated regions (red and dark yellow circles and lines), while it virtually disappears above regions without intercalant (green and blue circles and lines).

# 2 Theory

## Details of the Density Functional Theory (DFT) Modeling

Following Andersen *et al.*,[4] the optB88-vdW functional[5] and plane-wave calculations[6] were used to relax the sample structures. A slab of four Ir(111) layers entered into the simulations.

For graphene a $(6 \times 6)$ unit cell was used together with a $2 \times 2$ k-point sampling. The Ir slab was kept fixed and strained by $\approx 2\,\%$ to match the graphene unit cell dimensions, while the intercalant (Cs or Li) and graphene were relaxed. For Cs the distance between Ir and graphene is $630 \pm 7\,\mathrm{pm}$, while it is $430 \pm 8\,\mathrm{pm}$ in the case of Li (the ranges indicate the rippling), in reasonable agreement with previous findings.[4] In both cases we find a considerable $n$-doping corresponding to a Fermi energy of $\varepsilon_\mathrm{F} \approx 1\,\mathrm{eV}$.

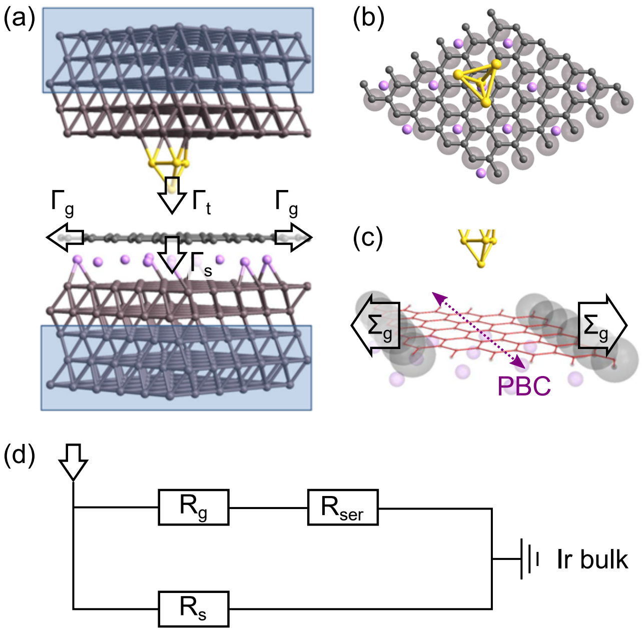


Figure S3: (a) Setup of the transport calculation for the example of Li. The Au tip atom is 440 pm above the graphene plane. Electrodes are attached at the slab regions indicated by the shaded areas. Schematically, electron escape rates to the tip, $\Gamma_\mathrm{t}$, to graphene, $\Gamma_\mathrm{g}$, and to the substrate, $\Gamma_\mathrm{s}$, are considered. (b) Tip and sample unit cell seen from above. (c) The three-terminal setup where electrons can terminate in the tip, graphene or the Ir substrate electrode. The graphene terminal is introduced in the calculations by using a pristine-graphene self-energy ($\mathbf{\Sigma}_\mathrm{g}$, marked by cirles) in the indicated directions in the graphene plane instead of periodic boundary conditions (PBC). PBC are used in the remaining direction in the graphene plane (dashed arrow). (d) Simple resistor picture for the electron transport from the tip to the bulk Ir electrode. The current injected into the graphene plane (represented by the resistance $R_\mathrm{g}$) outside the unit cell will eventually end up in the Ir bulk electrode ($R_\mathrm{s}$) *via* a series resistance ($R_\mathrm{ser}$).

The relaxed structures served as an input to the subsequent nonequilibrium Green function (NEGF) calculations. The SIESTA code[7] combined with the TRANSIESTA method,[8,9] and the INELASTICA package[10] to obtain the electron-phonon couplings *via* finite displacements

of the atoms were applied. To this end, Ir electrodes were attached to the relaxed structures and a small Au tip was mounted (Figure S3a, b). The Perdew-Burke-Ernzerhof (PBE) functional[11] with the standard single-zeta polarized (SZP) linear combination of atomic orbitals (LCAO) basis[7] was used for the Ir, the double-zeta polarized (DZP) basis for the outermost Ir layer and for the intercalants, and for graphene a double-zeta double-polarized (DZDP) basis set with range up to 0.45 nm, which includes the lowest unoccupied bands of graphene.[12,13]

## Multi-electrode Setup

We emphasize that the boundary conditions for the electron transport are crucial for describing the experiments. In a standard inelastic DFT-NEGF calculation one typically considers two terminals, the tip and Ir substrate, and uses periodic boundary conditions (PBC) in the transverse direction on the total structure. For large unit cells as in the present case one will typically use only a few transverse k-points. However, this setup results in vanishing vibrational signatures in the current and does not reproduce the experimental results.

In order to model the experimental data, where the inelastic conductance steps are of the same order of magnitude as the zero-bias conductance, it is important to resolve the states at the Fermi level in graphene. Instead of using a prohibitively fine transverse k-point sampling an alternative approach is proposed here by attaching a third terminal corresponding to freely propagating electrons in a graphene layer with a strong $n$-doping given by the graphene inside the cell. This amounts to replacing the PBC by open boundary conditions in one graphene direction, which is equivalent to introducing a graphene self-energy ($\mathbf{\Sigma}_{\mathrm{g}}$ in Figure S3c) as done in DFT-NEGF transport calculations.[8,9]

We calculate $\mathbf{\Sigma}_{\mathrm{g}}$ for a pristine graphene cell with the same parameters as in the full cell and fix the energy of $\mathbf{\Sigma}_{\mathrm{g}}$ to that of the Fermi energy of intercalated graphene. The PBC are kept in the remaining transverse direction for computational simplicity, and the Γ-point approximation is used like for the Ir electrodes in both transverse directions. Thus,

the electrons in graphene can couple with effective rates $\Gamma_\mathrm{t}$, $\Gamma_\mathrm{g}$, and $\Gamma_\mathrm{s}$ to, respectively, the tip, graphene outside the central cell, and the substrate as shown in Figure S3a, although these rates are not directly available or defined in the full calculation. A benefit of this approach is the possibility of evaluating the current that branches into the graphene under the tip, escapes into graphene, and only at some later stage enters into the bulk metal electrode away from the tip region (Figure S3a). We find that to a good approximation the total conductance equals the sum of the conductances of the graphene and the Ir substrate terminal. In a simple picture our setup can, therefore, be visualized as two resistors in parallel as depicted in Figure S3d, with an additional serial resistance $R_\mathrm{ser}$ for electrons, which enter the substrate only outside the unit cell.

## Calculation of Inelastic Electron Transport

The inelastic contribution to the current is obtained from the lowest-order expansion (LOE) method.[14] The expressions can easily be split into contributions from each of the terminals, *e. g.*, from graphene and Ir ($\alpha$), assuming the same chemical potential in graphene and Ir. Following a previous report,[14] the contribution of each terminal $\alpha$ for a given mode $\kappa$ is calculated as

$$\begin{aligned}\partial_V^2 I^\alpha(V) &= (\gamma_{i,\kappa} + \mathrm{Im}B_\kappa^\alpha)\,\partial_V^2\mathcal{I}^\mathrm{sym}(V,\hbar\omega_\kappa,T,N_\kappa)\\ &\quad + (2\mathrm{Re}B_\kappa^\alpha)\,\partial_V^2\mathcal{I}^\mathrm{asym}(V,\hbar\omega_\kappa,T),\end{aligned} \tag{1}$$

where the constants are given in terms of Green functions ($\mathbf{G}$), spectral functions ($\mathbf{A}$), and electron-phonon couplings ($\gamma$)

$$\begin{aligned}B_\kappa^\alpha \equiv \mathrm{Tr}[&\mathbf{\Gamma}_\alpha(\mu_L)\,\mathbf{G}(\mu_L)\mathbf{M}_\kappa\mathbf{A}_R(\mu_R)\mathbf{M}_\kappa\mathbf{A}_R(\mu_L)\\ &- \mathbf{\Gamma}_\alpha(\mu_R)\,\mathbf{A}_R(\mu_R)\mathbf{M}_\kappa\mathbf{A}_L(\mu_L)\mathbf{M}_\kappa\mathbf{G}^\dagger(\mu_R)],\end{aligned} \tag{2}$$

and

$$\gamma^{\alpha}_{i,\kappa} = \mathrm{Tr}\big[\mathbf{\Gamma}_{\alpha}(\mu_L)\,\mathbf{G}(\mu_L)\mathbf{M}_{\kappa}\mathbf{A}_R(\mu_R)\mathbf{M}_{\kappa}\mathbf{G}^{\dagger}(\mu_L)\big] \tag{3}$$

with the chemical potentials $\mu_L$, $\mu_R$ for, respectively, left and right electrode. We use an energy constant $\mathbf{\Gamma}$ in graphene (due to the artificial PBC in one direction) and consider only the voltage-symmetric part of the conductance. Furthermore, contributions from Ir phonons ($< 20\,\mathrm{meV}$) are neglected, and only vibrations of the C atoms are included. The central inelastic scattering region in the calculation setting the size of the $\sigma$–$\pi$ coupling matrix $\mathbf{M}$ includes two layers of Ir on both sides (Figure S3).

## Contributing Phonon Modes

In order to analyze the phonon modes that dominantly contribute to the inelastic current we project these onto graphene phonons of the primitive unit cell in the following way, which has been inspired by the effective band structures for alloys.[15] Using the (6×6) graphene supercell for the simulation of intercalated graphene the approximate band structure is formed by averaging the supercell dynamical matrix over unit cells separated by linear combinations of the primitive real space unit vectors.

The primitive k-points corresponding to the supercell and Brillouin zone are shown in Figure S4a along with the effective phonon band structure in Figure S4b. The degeneracy of the primitive graphene bands is lifted due to the substrate interaction as seen in the slightly different bands when taking round trips $\Gamma$–$M$–$K$–$\Gamma$ in the Brillouin zone.

On top of the bands we show circles at the mode energies and at k-points where the overlap is large (Figure S4b). The radius is proportional to the IETS signal for the mode and k-mode overlap (shown for Cs at a junction conductance of $G = 0.02\,\mathrm{G}_0$). We see that the phonons are mainly due to modes similar to out-of-plane phonons at $K$ and $M$, but the breaking of symmetry yields contributions shifted away from these, mainly from the k-point close to the middle of the $M$–$K$ direction (marked k-point in Figure S4a).

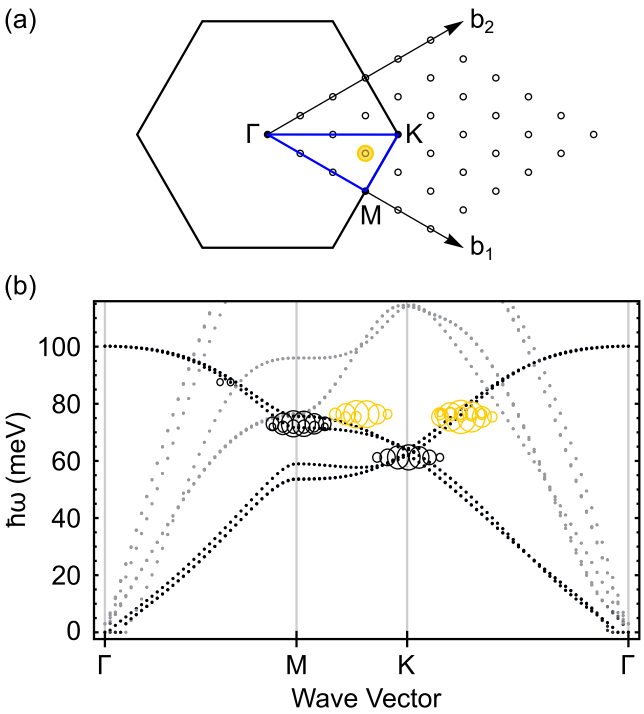


Figure S4: (a) The graphene Brillouin zone with high-symmetry points Γ, $M$, $K$ is spanned by reciprocal lattice vectors $\mathbf{b}_1$ and $\mathbf{b}_2$. The circles mark the k-points of the $(6 \times 6)$ supercell. The k-point marked with a yellow circle is contributing to the inelastic signals besides $M$ and $K$. (b) Phonon modes projected onto the effective band structure for the graphene unit cell. The black (gray) bands depict the dispersion of out-of-plane (in-plane) phonons. The circles are placed at the phonon energy $\hbar\omega$ with a radius scaled by the k-projection overlap and IETS signal strength. The contributions in yellow stem from the k-point marked in (a). Only phonon modes with strongest contributions are shown.

## Simple Model

The findings obtained by the DFT-NEGF calculation can be expressed in a simplified two-level model involving a $\pi$ state at $K/K'$ with energy ($\varepsilon_\pi = \varepsilon_\mathrm{F} \approx 0\,\mathrm{eV}$) and a $\sigma$ state representing the first unoccupied band at Γ with energy $\varepsilon_\sigma$. This model is inspired by a previous work,[12] although the $\sigma$ state in principle could also represent a tip $s$ state.

The wide-band approximation is used and the coupling of the graphene $\pi$ state to the substrate is modeled by an imaginary self-energy (inverse lifetime) $\Gamma_\pi$. The $\sigma$ state is also coupled to the substrate *via* $\Gamma_\sigma$ as well as to the tip *via* $\Gamma_\mathrm{t}$. The $\sigma$ state has a long range[13] and, thus, $\Gamma_\sigma > \Gamma_\pi$. Considering now that the current can flow directly between the tip, $\sigma$ state and the substrate, or from the tip, $\sigma$ state *via* phonon excitation (electron-phonon

coupling $\lambda$) to the graphene $\pi$ state and subsequently to the substrate, the corresponding unperturbed (no phonon) Green function reads

$$\mathbf{G} = \begin{pmatrix} \varepsilon - \mathrm{i}\frac{\Gamma_\pi}{2} & 0 \\ 0 & \varepsilon - \varepsilon_\sigma - \mathrm{i}\frac{\Gamma_\mathrm{t}+\Gamma_\sigma}{2} \end{pmatrix}^{-1} . \tag{4}$$

The phonon couples the $\sigma$ and $\pi$ state by the matrix

$$\mathbf{M} = \lambda \begin{pmatrix} 0 & 1 \\ 1 & 0 \end{pmatrix} . \tag{5}$$

For the inelastic process the lowest-order (symmetric) inelastic conductance step height is [14,16]

$$\gamma = \mathrm{Tr}[\mathbf{M}\tilde{\mathbf{A}}_L \mathbf{M}\mathbf{A}_R] \tag{6}$$

with $\mathbf{A}_R = \mathbf{G}^\dagger \mathbf{\Gamma}_R \mathbf{G}$ ($\tilde{\mathbf{A}}_L = \mathbf{G}\mathbf{\Gamma}_L\mathbf{G}^\dagger$), $\mathbf{A}_R$ ($\tilde{\mathbf{A}}_L$) being the right (left time-reversed) spectral function. The right electrode $R$ may represent the tip,

$$\mathbf{\Gamma}_R = \begin{pmatrix} 0 & 0 \\ 0 & \Gamma_\mathrm{t} \end{pmatrix} \tag{7}$$

while the left electrode L represents the substrate,

$$\mathbf{\Gamma}_L = \begin{pmatrix} \Gamma_\pi & 0 \\ 0 & \Gamma_\sigma \end{pmatrix} . \tag{8}$$

The inelastic step height reads

$$\gamma = \lambda^2 A_\pi(\varepsilon_\mathrm{F} + \hbar\Omega) A_\sigma(\varepsilon_\mathrm{F}) \tag{9}$$

where ($\varepsilon_{\rm F} \equiv 0\,{\rm eV}$),

$$A_\sigma(\varepsilon_{\rm F}) = \frac{\Gamma_{\rm t} + \Gamma_\sigma}{\varepsilon_\sigma^2 + \left(\frac{\Gamma_{\rm t}}{2} + \frac{\Gamma_\sigma}{2}\right)^2}, \tag{10}$$

and

$$A_\pi(\varepsilon_{\rm F}) = \frac{\Gamma_\pi}{(\hbar\Omega)^2 + \left(\frac{\Gamma_\pi}{2}\right)^2}. \tag{11}$$

Likewise, the zero-bias conductance is obtained as

$$g(0) = {\rm Tr}[\mathbf{\Gamma}_L \mathbf{A}_R] = \frac{\Gamma_{\rm t}\,\Gamma_\sigma}{\varepsilon_\sigma^2 + \left(\frac{\Gamma_{\rm t}}{2} + \frac{\Gamma_\sigma}{2}\right)^2}. \tag{12}$$

If we assume $\hbar\Omega \ll \Gamma_\pi$ and neglect the vibrational energy we can now calculate the relative conductance increase (inelastic step height divided by the zero bias conductance),

$$\frac{\Delta g}{g(0)} = \frac{\gamma}{g(0)} = \frac{4\lambda^2}{\Gamma_\pi}\left(\frac{1}{\Gamma_{\rm t}} + \frac{1}{\Gamma_\sigma}\right). \tag{13}$$

For small tip coupling $\Gamma_{\rm t} \ll \Gamma_\sigma$ we obtain

$$\frac{\gamma}{g(0)} = \frac{4\lambda^2}{\Gamma_{\rm t}\Gamma_\pi}. \tag{14}$$

This explains why for increased hybridization of graphene with the substrate or increased tip–graphene coupling, the inelastic signals become quenched in the experiments.

In the limit of very small substrate coupling ($\Gamma_\pi, \Gamma_\sigma \ll \hbar\Omega, \Gamma_{\rm t}$)

$$\frac{\gamma}{g(0)} = \frac{\lambda^2}{(\hbar\Omega)^2}\frac{\Gamma_\pi}{\Gamma_\sigma}, \tag{15}$$

where now the coupling $\Gamma_\pi$ becomes a bottle-neck for the inelastic process.

When the tip is in direct contact with graphene we may expect $\Gamma_{\rm t} \gg \Gamma_\sigma$ and thus

$$\frac{\gamma}{g(0)} = \frac{4\lambda^2}{\Gamma_\sigma\Gamma_\pi}. \tag{16}$$

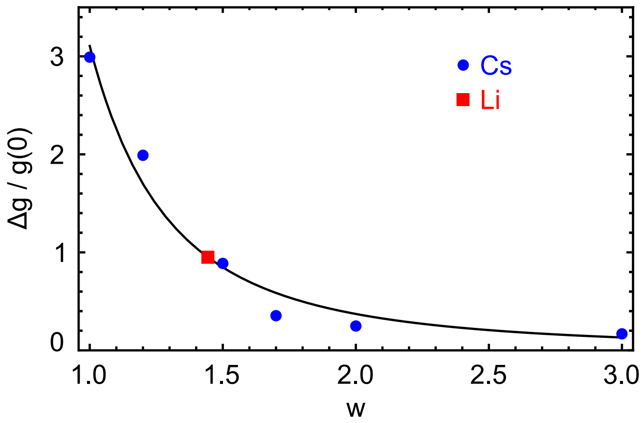


Figure S5: Fit (solid line) of eq 17 to the DFT results for Cs (dots), where the Hamiltonian matrix element, $w$, between C and Ir atoms was scaled by hand. The unscaled Li data point (square) is shown for comparison.

Assuming that $\Gamma_\sigma$ and $\Gamma_\pi$ scale in the same way as we change the distance to the substrate, we get a scaling with substrate Hamiltonian matrix element, $w$, $\Gamma_\pi \propto \Gamma_\sigma \propto w^2$,

$$\frac{\gamma}{g(0)} \propto \frac{1}{w^2}\left(1+\frac{a}{w^2}\right), \tag{17}$$

where $a$ is the ratio $\Gamma_\mathrm{t}/\Gamma_\sigma$ at $w=1$. In Figure S5 we show the fit of this expression to the DFT results.

To obtain a simple measure of the coupling to the $\pi$ orbitals directly from the DFT-NEGF calculation we calculate

$$\Gamma_\pi = \frac{\mathrm{Tr}[\mathbf{S}\,(\mathbf{P}_\pi \mathbf{A}(E_F)\mathbf{P}_\pi)\,\mathbf{P}_\pi \boldsymbol{\Gamma}(E_F)\mathbf{P}_\pi]}{\mathrm{Tr}[\mathbf{S}\,(\mathbf{P}_\pi \mathbf{A}(E_F)\mathbf{P}_\pi)]} \tag{18}$$

where $\mathbf{P}_\pi$ is the projection matrix onto the $\pi$-electronic system of graphene. Here, the broadening of the $\pi$ states is estimated by projecting the broadening matrix, $\boldsymbol{\Gamma}$, obtained from the self-energy of the entire intercalated sample, weighted by graphene $p_z$-states via the projection of the spectral density ($\mathbf{A}$) at the Fermi level, to the $\pi$ system (and including the non orthogonality via the overlap matrix, $\mathbf{S}$). This procedure yields a lifetime broadening of $\Gamma_\pi = 0.67\,\mathrm{eV}$ for Li and $\Gamma_\pi = 0.18\,\mathrm{eV}$ for Cs, which is in good agreement with the ratio of $\Delta g(\mathrm{Cs})/\Delta g(\mathrm{Li}) \approx 3 \approx \Gamma_\pi(\mathrm{Li})/\Gamma_\pi(\mathrm{Cs})$ for similar $\Gamma_\mathrm{t}$ (tip distances). From the simple fit

procedure (Figure S5) $\lambda$ and $\Gamma_\sigma$ can be estimated. The fit yields $\Gamma_t/\Gamma_\sigma = a \approx 2.3$. Using $g_0 = 0.02\, G_0$ in eq 12 and $\Delta g/g_0 \approx 3$ in eq 13 leads to $\Gamma_\sigma = 0.35\,\mathrm{eV}$ for Cs and $\lambda = 0.18\,\mathrm{eV}$ for both intercalants. Consequently, for Li the coupling is scaled to $\Gamma_\sigma = 3 \cdot 0.35\,\mathrm{eV} = 1.05\,\mathrm{eV}$. These results are summarized in Table S1 below.

Table S1: Coupling constants for the calculated Cs and Li systems obtained from the fitting procedure described in the text.

| | $\Gamma_\sigma$ (eV) | $\Gamma_\pi$ (eV) | $\lambda$ (eV) |
|---|---|---|---|
| Cs | 0.35 | 0.18 | 0.18 |
| Li | 1.05 | 0.67 | 0.18 |

# References


(1) Hattab, H.; N'Diaye, A. T.; Wall, D.; Jnawali, G.; Coraux, J.; Busse, C.; van Gastel, R.; Poelsema, B.; Michely, T.; zu Heringdorf, F.-J. M.; von Hoegen, M. H. Growth temperature dependent graphene alignment on Ir(111). *Appl. Phys. Lett.* **2011**, *98*, 141903.

(2) Halle, J.; Néel, N.; Kröger, J. Filling the Gap: Li-Intercalated Graphene on Ir(111). *J. Phys. Chem. C* **2016**, *120*, 5067–5073.

(3) Petrović, M. et al. The mechanism of caesium intercalation of graphene. *Nat. Commun.* **2013**, *4*, 2772.

(4) Andersen, M.; Hornekær, L.; Hammer, B. Understanding intercalation structures formed under graphene on Ir(111). *Phys. Rev. B* **2014**, *90*, 155428.

(5) Klimeš, J.; Bowler, D. R.; Michaelides, A. Chemical accuracy for the van der Waals density functional. *J. Phys.: Condens. Matter* **2010**, *22*, 022201.

(6) Kresse, G.; Furthmüller, J. Efficiency of ab-initio total energy calculations for metals and semiconductors using a plane-wave basis set. *Comput. Mater. Sci.* **1996**, *6*, 15 – 50.

(7) Soler, J. M.; Artacho, E.; Gale, J. D.; García, A.; Junquera, J.; Ordejón, P.; Sánchez-Portal, D. The SIESTA method for ab initio order- N materials simulation. *J. Phys.: Condens. Matter* **2002**, *14*, 2745–2779.

(8) Brandbyge, M.; Mozos, J.-L.; Ordejón, P.; Taylor, J.; Stokbro, K.; Ordejo, P. Density-functional method for nonequilibrium electron transport. *Phys. Rev. B* **2002**, *65*, 165401.

(9) Papior, N.; Lorente, N.; Frederiksen, T.; García, A.; Brandbyge, M. Improvements on non-equilibrium and transport Green function techniques: The next-generation TRANSIESTA. *Comput. Phys. Commun.* **2017**, *212*, 8 – 24.

(10) Frederiksen, T.; Paulsson, M.; Brandbyge, M.; Jauho, A.-P. Inelastic transport theory from first principles: Methodology and application to nanoscale devices. *Phys. Rev. B* **2007**, *75*, 205413.

(11) Perdew, J. P.; Burke, K.; Ernzerhof, M. Generalized Gradient Approximation Made Simple. *Phys. Rev. Lett.* **1996**, *77*, 3865–3868.

(12) Wehling, T. O.; Grigorenko, I.; Lichtenstein, A. I.; Balatsky, A. V. Phonon-Mediated Tunneling into Graphene. *Phys. Rev. Lett.* **2008**, *101*, 216803.

(13) Papior, N. R.; Calogero, G.; Brandbyge, M. arXiv:1803.01568.

(14) Lü, J.-T.; Christensen, R. B.; Foti, G.; Frederiksen, T.; Gunst, T.; Brandbyge, M. Efficient calculation of inelastic vibration signals in electron transport: Beyond the wide-band approximation. *Phys. Rev. B* **2014**, *89*, 081405.

(15) Popescu, V.; Zunger, A. Effective band structure of random alloys. *Phys. Rev. Lett.* **2010**, *104*, 236403.

(16) Paulsson, M.; Frederiksen, T.; Brandbyge, M. Inelastic Transport through Molecules: Comparing First-Principles Calculations to Experiments. *Nano Lett.* **2006**, *6*, 258–262.
